# Supplementary material for: Inferring the finest pattern of mutual independence from data
Source: arXiv:2306.12984 ancillary file (2023-06-22)
Supplement: Supplementary file 1 [file SupplementaryMaterial.pdf]

# Supplementary material for manuscript “Inferring the finest pattern of mutual independence from data”

G. Marrelec and A. Giron

## Contents

|          |                                                              |          |
|----------|--------------------------------------------------------------|----------|
| <b>1</b> | <b>The lattice of partitions</b>                             | <b>1</b> |
| <b>2</b> | <b>Simulation study: correlation thresholding</b>            | <b>3</b> |
| <b>3</b> | <b>Simulation study: noncentral chi-squared distribution</b> | <b>4</b> |

## 1 The lattice of partitions

We here quickly review the main features of  $\Omega(N)$  as a lattice based on Birkhoff (1973, Chap. 1), Aigner (1979, Chap. I, §2.B) and Knuth (2004).

On the set of partitions  $\Omega(N)$ , one can define the following relation:  $\pi$  is a finer partition than (or a refinement of)  $\omega$ , denoted  $\pi \leq \omega$ , if every block of  $\pi$  is contained in a block of  $\omega$ . If  $\pi$  is finer than  $\omega$ , then  $\omega$  is said to be coarser than  $\pi$ . The relation “ $\leq$ ” has 3 properties:

- reflexivity: for all  $\pi$ ,  $\pi \leq \pi$ ;
- antisymmetry: if  $\pi \leq \omega$  and  $\omega \leq \pi$  then  $\pi = \omega$ ;
- transitivity: if  $\pi \leq \omega$  and  $\omega \leq \rho$ , then  $\pi \leq \rho$ .

$\Omega(N)$  is therefore called a partially ordered set, or poset.

If  $\pi \leq \omega$  and  $\pi \neq \omega$ , we write  $\pi < \omega$ . If  $\pi < \omega$  and there does not exist a  $\rho$  such that  $\pi < \rho < \omega$ , we say that  $\omega$  covers  $\pi$ , written  $\pi \prec \omega$ .  $\omega$  is then a direct successor to  $\pi$  in the hierarchy induced by  $\leq$ . In  $\Omega(N)$ ,  $\omega$  covers  $\pi$  if  $\omega$  is obtained by merging two blocks of  $\pi$ .

In  $\Omega(N)$ , the partition  $O = 1 \mid 2 \mid \dots \mid N$  is such that  $O \leq \pi$  for all  $\pi \in \Omega(N)$ . It is called the least element, or bottom, of  $\Omega(N)$ . Dually,  $I = 12 \dots N$  is such that  $\pi \leq I$  for all  $\pi \in \Omega(N)$ . It is called the greatest element, or top, of  $\Omega(N)$ .  $O$  and  $I$  are called universal bounds of  $\Omega(N)$  as  $O \leq \pi \leq I$  for all  $\pi \in \Omega(N)$ . The elements that cover the bottom are called the atoms. In  $\Omega(N)$ , there are  $N(N-1)/2$  atoms, each one with  $N-2$  blocks of size 1 and 1 block of size 2, e.g.,  $12 \mid 3 \mid \dots \mid N$  or  $1 \mid 23 \mid 4 \mid \dots \mid N$ .

Given a pair of partitions  $\pi$  and  $\omega$ , their upper bound is defined as the set of all  $\rho$  such that  $\pi \leq \rho$  and  $\omega \leq \rho$ . In  $\Omega(N)$ , a unique least upper bound exists, called the join and written  $\pi \vee \omega$ . Similarly, we can define the lower bound as the set of all  $\rho$  such that  $\rho \leq \pi$  and  $\rho \leq \omega$ . In  $\Omega(N)$ , a unique greatest lower bound exists, called the meet and written  $\pi \wedge \omega$ . In particular, we have for the top partition  $I$ , bottom partition  $O$  and all  $\pi \in \Omega(N)$ ,

$$O \wedge \pi = O, \quad O \vee \pi = \pi, \quad I \wedge \pi = \pi, \quad \text{and} \quad I \vee \pi = I. \quad (1)$$

Besides, the consistency relationship expresses the relationship between the ordering and the join and meet operators:

$$\pi \leq \omega \quad \Leftrightarrow \quad \begin{cases} \pi \wedge \omega = \pi \\ \pi \vee \omega = \omega. \end{cases} \quad (2)$$

Practically, the meet  $\pi \wedge \omega$  of  $\pi = a_1 \mid \cdots \mid a_k$  and  $\omega = b_1 \mid \cdots \mid b_l$  is the partition that has blocks  $a_i \cap b_j$  for any  $1 \leq i \leq k$  and  $1 \leq j \leq l$  such that  $a_i \cap b_j \neq \emptyset$ . In this definition, “ $\cap$ ” stands for the usual set intersection. In other words, two elements of  $N$  belong to the same block of  $\pi \wedge \omega$  if and only if they do for both  $\pi$  and  $\omega$ .

The concept of covering can be used to provide a graphical representation of  $\Omega(N)$ . If  $\pi \leq \omega$ , then  $\omega$  is drawn higher than  $\pi$  in the diagram. If  $\pi \prec \omega$  then  $\pi$  and  $\omega$  are connected through a line. See for instance Figure 1 for a representation of  $\Omega([3])$  and  $\Omega([4])$ .

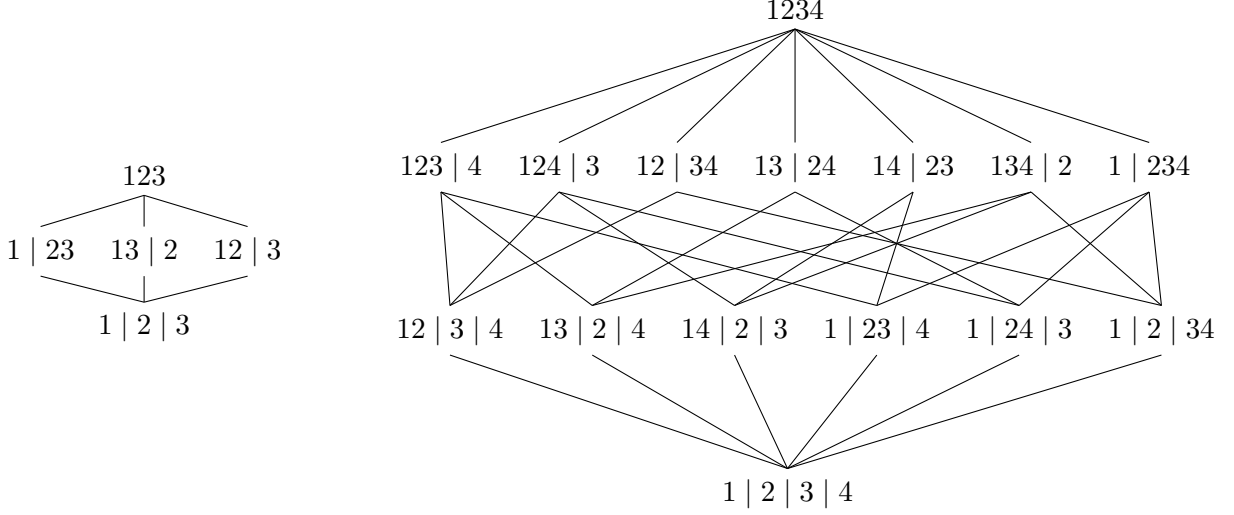

Figure 1: **Examples of partition lattices.** Representation of  $\Omega([3])$  (left) and  $\Omega([4])$  (right).

Since  $\Omega(N)$  is a poset for which the join ( $\vee$ ) and meet ( $\wedge$ ) exist for every pair of partitions, it is called a lattice. In lattices, the join and meet have the following properties:

- idempotency:  $\pi \wedge \pi = \pi$  and  $\pi \vee \pi = \pi$ ;
- commutativity:  $\pi \wedge \omega = \omega \wedge \pi$  and  $\pi \vee \omega = \omega \vee \pi$ ;
- associativity:  $(\pi \wedge \omega) \wedge \rho = \pi \wedge (\omega \wedge \rho)$  and  $(\pi \vee \omega) \vee \rho = \pi \vee (\omega \vee \rho)$ ;
- absorption:  $\pi \wedge (\pi \vee \omega) = \pi$  and  $\pi \vee (\pi \wedge \omega) = \pi$ .

We also have the following properties:

$$\omega \leq \rho \quad \Rightarrow \quad \begin{cases} \pi \wedge \omega \leq \pi \wedge \rho \\ \pi \vee \omega \leq \pi \vee \rho. \end{cases} \quad (3)$$

Note that  $\Omega(N)$  is not distributive.

## 2 Simulation study: correlation thresholding

We independently tested each sample correlation coefficient  $r$  under the null hypothesis that it is equal to 0 using the fact that, under this assumption,

$$\frac{r\sqrt{k-2}}{\sqrt{1-r^2}} \quad (4)$$

has the  $t$ -distribution with  $k-2$  degrees of freedom (Anderson, 1958, §4.2.1). We then performed multiple comparison using the FDR approach as detailed in §3.3.2 of the manuscript (Benjamini and Hochberg, 1995). The finest pattern of mutual independence was finally obtained by identifying each block with a maximally connected component. Results regarding the ratio of correct inference at a significance level of  $\alpha = 0.1$  are summarized in Figure 2.

Note that we did not compute the other quantities presented in Figure 2 of the manuscript, such as AUC, sensitivity and specificity. While we could compute them, their use as a way to compare approaches would be very limited. Indeed, in the case of our approach, these quantities were calculated using the rates of true/false positive/negatives among the set  $\Omega_2(N)$  of dichotomic independence relationships, which has a cardinality of  $2^{n-1} - 1$ . By contrast, in the case of correlation thresholding, they could only be calculated using the rates of true/false positive/negatives among the set of correlation coefficients, which has a cardinality of  $n(n-1)/2$ .

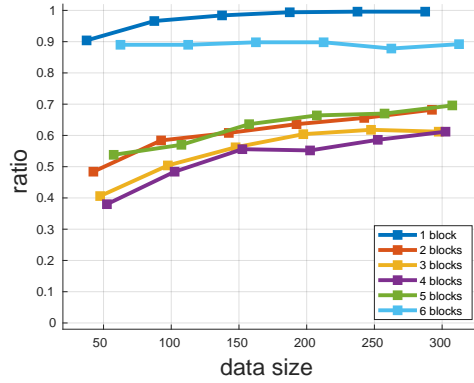

Figure 2: **Simulation study.** For a significance level  $\alpha = 0.1$ , ratio of patterns of mutual independence correctly detected using correlation thresholding and FDR.

### 3 Simulation study: noncentral chi-squared distribution

We used the same procedure as detailed in §4.2 of the manuscript, except for the fact that we used the noncentral chi-squared approximation developed in §3.3.1 of the manuscript. Results are reported in Figure 3.

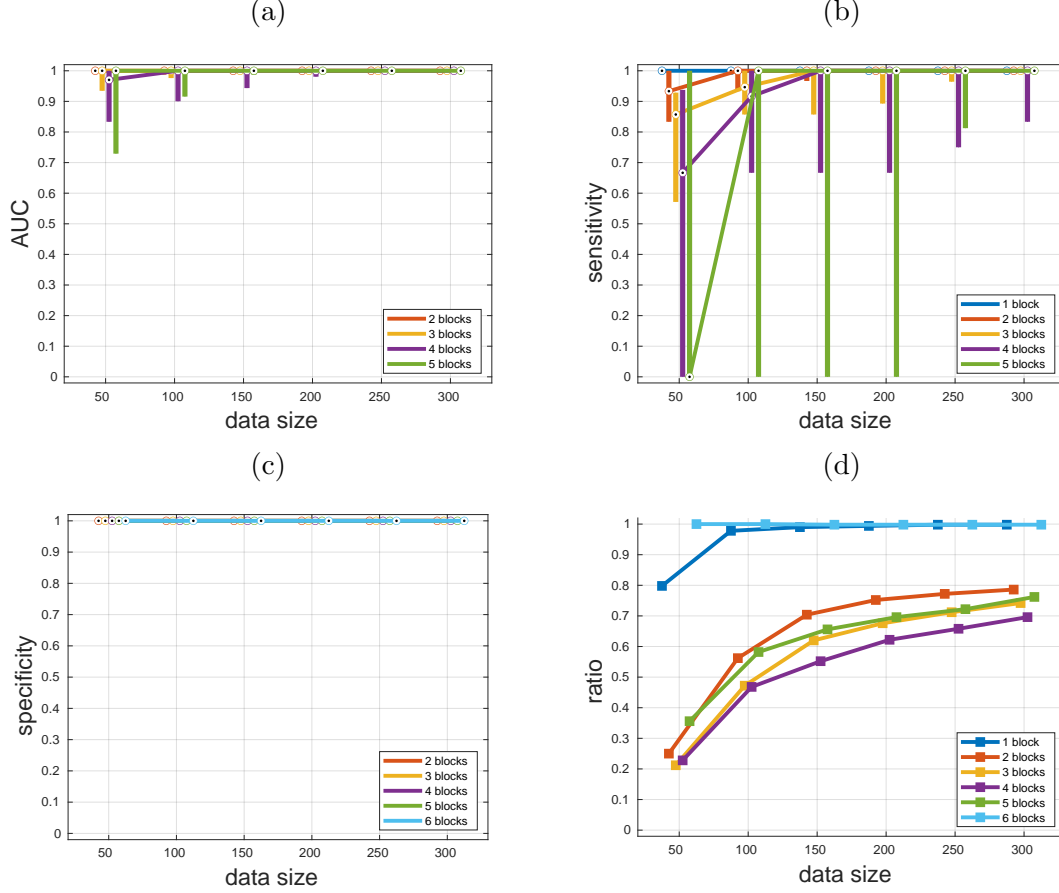

Figure 3: **Simulation study.** (a) AUC. For a significance level  $\alpha = 0.1$ : (b) Sensitivity; (c) Specificity. (d) Ratio of patterns of mutual independence correctly detected. (a), (b) and (c) are boxplot (median and [25%, 75%] frequency interval).  $p$ -values are computed with noncentral chi-squared distribution.

## References

- Aigner, M., 1979. Combinatorial Theory. volume 234 of *Grundlehren der mathematischen Wissenschaften*. Springer, Berlin.
- Anderson, T.W., 1958. An Introduction to Multivariate Statistical Analysis. Wiley Publications in Statistics, John Wiley and Sons, New York.
- Benjamini, Y., Hochberg, Y., 1995. Controlling the false discovery rate: a practical and powerful approach to multiple testing. *Journal of the Royal Statistical Society: Series B (Statistical Methodology)* 57, 289–300.
- Birkhoff, G., 1973. Lattice Theory. volume XXV of *American Mathematical Society Colloquium Publications*. 3rd ed., American Mathematical Society, Providence, Rhode Island.

Knuth, K.H., 2004. Lattice duality: the origin of probability and entropy. *Neurocomputing* 67, 245–274.
